# Supplementary material for: Human-3Diffusion: Realistic Avatar Creation via Explicit 3D Consistent Diffusion Models
Source: arXiv:2406.08475 source file (2024-12-14)
Supplement: Supplementary file 1 [file supp_implementation.tex]

\subsection{Implementation Details}
